# Supplementary material for: Renormalisation group running effects in $pp\to t\bar{t}h$ in the Standard Model Effective Field Theory
Source: arXiv:2312.11327 source file (2024-04-26)
Supplement: Supplementary file 1 [file AdditionalPreamble.tex]

%Stuff added by me 

%rientro della prima riga di ogni capoverso 
%\setlength\parindent{0pt}


\usepackage{csquotes} 
%\usepackage[style=numeric, %numeric labels assigned to the entries in the bibliography
%sortcites,  %multiple citations are sorted, e.g. \cite{ref2,ref1} gives [1,2]
%citestyle=numeric-comp, % [1,2,3] -> [1-3]
%sorting=none, %sorting in the bibliography
%none = order of citation 
%hyperref]{biblatex}
%\addbibresource{Biblio1.bib}
%\usepackage[nottoc,numbib]{tocbibind}



\usepackage{slashed} %feynman slash notation 
\usepackage{subcaption} %[labelfont=up]

%for diagrams 
\usepackage{tikz}
\usetikzlibrary{shapes.geometric}
%\usetikzlibrary{shapes}
\usepackage[compat=1.1.0]{tikz-feynman} %Feynman diagrams

\usepackage{comment}
\usepackage{alltt}
%\usepackage{minted} %To display terminal output
\usepackage{fancyvrb}

\usepackage{braket}
\usepackage{amssymb, amsmath, mathtools,slashed, breqn, amsthm, mathrsfs, esint, bm}

\usepackage{listings}

\lstset{
	upquote=true, %to correctly reproduce ` instead of 's
	backgroundcolor=\color{gray!10},  
	basicstyle=\ttfamily,
	belowskip=-0.95 \baselineskip,
	aboveskip=\bigskipamount,
	columns=fullflexible,
	breakatwhitespace=false,      
	breaklines=true,                
	captionpos=b,                    
	commentstyle=\color{green}, 
	extendedchars=true,              
	frame=single,                   
	keepspaces=false,             
	keywordstyle=\color{blue},      
	language=c++,                 
	numbers=none,                
	numbersep=5pt,                   
	numberstyle=\tiny\color{blue}, 
	rulecolor=\color{gray},    
	%To show spaces as the small symbol set these two to true    
	showspaces=false,              
	showstringspaces=false,                
	showtabs=false,                 
	stepnumber=5,                  
	stringstyle=\color{purple},    
	tabsize=3,                      
	title=\lstname                
}



\usepackage{float}
